# Supplementary material for: Progressive Token Length Scaling in Transformer Encoders for Efficient Universal Segmentation
Source: arXiv:2404.14657 source file (2025-03-29)
Supplement: Supplementary file 1 [file supp_error_bars.tex]

\begin{table}[!t]
	
	\setlength{\tabcolsep}{5pt}
	\begin{minipage}{.5\linewidth}
		\caption[Random seed evaluations with error bars for \ours]{Random seed evaluations for \ours (s.e. = standard error)}
		\centering
		\resizebox{0.85\textwidth}{!}{
	\label{tab:random_runs}
	\begin{tabular}{rccc}
		\hline
		\rowcolor[HTML]{EFEFEF} 
		& \textbf{PQ} & \textbf{mIoU}$_p$ & \textbf{AP}$_p$ \\
		\hline
		Run 1  & 52.90  & 63.22  & 42.78\\
		Run 2  & 53.05  & 63.50  & 42.72 \\
		Run 3  & 52.89 & 63.83 & 42.56 \\
		Run 4  & 52.80 & 63.22 & 42.38 \\
		Run 5  & 52.82 & 63.49 &  42.60 \\
		\midrule 
		\rowcolor[HTML]{E9FAFD} 
		mean & 52.89 & 63.45 & 42.61 \\
		\rowcolor[HTML]{E9FAFD} 
		s.e. & 0.06325 & 0.11251 & 0.06926 \\
		\hline 
	\end{tabular}
}
	\end{minipage}%
	\begin{minipage}{.5\linewidth}
		\centering
		\pgfplotstableread{
	x                   y     y-max 
	\text{PQ}      52.89    0.06325
	\text{mIoU}$_p$       63.45    0.11251  
	\text{AP}$_p$       42.61    0.06926
}{\mytable}

\pgfplotsset{compat=1.5, scaled y ticks=false}

% ============================

\pgfplotsset{
	every axis/.append style = {thick},tick style = {thick,black},
	y tick label style={
		/pgf/number format/.cd,
		fixed,
		fixed zerofill,
		precision=0,
		/tikz/.cd
	},
	%
	% #1 = x, y, or z
	% #2 = the shift value
	/tikz/normal shift/.code 2 args = {%
		\pgftransformshift{%
			\pgfpointscale{#2}{\pgfplotspointouternormalvectorofticklabelaxis{#1}}%
		}%
	},%
	range3frame/.style = {
		tick align        = outside,
		scaled ticks      = false,
		enlargelimits     = false,
		ticklabel shift   = {10pt},
		axis lines*       = left,
		line cap          = round,
		clip              = false,
		xtick style       = {normal shift={x}{20pt}},
		ytick style       = {normal shift={y}{10pt}},
		ztick style       = {normal shift={z}{10pt}},
		x axis line style = {normal shift={x}{10pt}},
		y axis line style = {normal shift={y}{10pt}},
		z axis line style = {normal shift={z}{10pt}},
	}
}

\begin{tikzpicture}[scale=0.75, transform shape]
	\begin{axis} [
		title={\large Error bars (with standard error)},
		symbolic x coords={\text{PQ}, \text{mIoU}$_p$, \text{AP}$_p$},
		xtick=data,
		ymajorgrids=true,
		axis background/.style={fill=trueblue!10},
		ylabel={\textcolor{red}{Performance (\%)}},
		xlabel={Segmentation Task (metric)},
		ytick={40,45,50,55,60,65},
		yticklabel={$\pgfmathprintnumber{\tick}\%$},
		]
		\addplot [only marks, red, fill=red] 
		plot [error bars/.cd, y dir=both, y explicit]
%		table [y error plus=y-max, y error minus=y-max] {\mytable};
		table [y=y, y error=y-max] {\mytable};
	\end{axis} 
\end{tikzpicture}
	\end{minipage}
\end{table}
