# Supplementary material for: Progressive Token Length Scaling in Transformer Encoders for Efficient Universal Segmentation
Source: arXiv:2404.14657 source file (2025-03-29)
Supplement: Supplementary file 4 [file 2_limitations_broader_impacts.tex]

\section{Limitations}
\label{sec:limitations}
Our approach assumes that the parent model's backbone provides multi-scale features as input to the encoder. However, this assumption might not hold true if the backbone is a standard vision transformer (ViT). In such cases, one could utilize feature pyramid networks to take advantage of multi-scale features while still benefiting from the efficiency gains offered by our approach.

\section{Broader Impact}
\label{sec:broader_impact}
Our research on efficient universal segmentation can help broaden the access to powerful segmentation models to users with limited compute availability. At the same time, it can have a positive impact in saving design costs for many real-world applications as an organization can customize \ours to meet different compute demands. Potential negative ethical aspects and future societal consequences are similar to ones associated with conventional deep learning models such as susceptibility to adversarial attacks, prediction fairness, issues with training dataset bias, \etc.
