# Supplementary material for: Progressive Token Length Scaling in Transformer Encoders for Efficient Universal Segmentation
Source: arXiv:2404.14657 source file (2025-03-29)
Supplement: Supplementary file 5 [file supp_add_fps_1.tex]

\caption{\ours \textbf{Ablation analysis with FPS }. Comparison of different configurations of \ours for PQ and FPS for the encoder with SWIN-T backbone on COCO dataset. \ours provides a flexible way to adjust performance and speed by varying its configuration factors.}
\centering
\resizebox{\columnwidth}{!}{%
\begin{tabular}{cccc}
	\toprule
	\textbf{Method} & \textbf{Setting} & \textbf{PQ} ($\uparrow$) & \textbf{FPS} ($\uparrow$) \\
	\midrule
%	 \multicolumn{4}{c}{\textbf{Cityscapes} }\\
%	 \midrule
%	\ours &  (1,1,1)  & 60.58 & 5.05 \\
%	\ours &  (2,2,2)  & 62.37 & 4.26 \\
%	\ours &  (3,3,3) & 63.06 & 4.12 \\
%	\midrule 
%	 \multicolumn{4}{c}{\textbf{COCO} }\\
%	 \midrule 
	\ours &  (1,1,1)  & 50.79 & 6.76 \\
	\ours &  (2,2,2) & 52.12 & 5.45 \\
	\ours &  (3,3,3) & 52.82 & 5.25 \\
	\bottomrule
\end{tabular}
}
\label{tab:supp_add_fps_1}
