# Supplementary material for: Progressive Token Length Scaling in Transformer Encoders for Efficient Universal Segmentation
Source: arXiv:2404.14657 source file (2025-03-29)
Supplement: Supplementary file 6 [file supp_table_random_runs.tex]

\resizebox{0.85\textwidth}{!}{
	\label{tab:random_runs}
	\begin{tabular}{rccc}
		\hline
		\rowcolor[HTML]{EFEFEF} 
		& \textbf{PQ} & \textbf{mIoU}$_p$ & \textbf{AP}$_p$ \\
		\hline
		Run 1  & 52.90  & 63.22  & 42.78\\
		Run 2  & 53.05  & 63.50  & 42.72 \\
		Run 3  & 52.89 & 63.83 & 42.56 \\
		Run 4  & 52.80 & 63.22 & 42.38 \\
		Run 5  & 52.82 & 63.49 &  42.60 \\
		\midrule 
		\rowcolor[HTML]{E9FAFD} 
		mean & 52.89 & 63.45 & 42.61 \\
		\rowcolor[HTML]{E9FAFD} 
		s.e. & 0.06325 & 0.11251 & 0.06926 \\
		\hline 
	\end{tabular}
}
